# Supplementary material for: Anomalous frequency and temperature dependent scattering and Hund's coupling in the almost quantum critical heavy fermion system CeFe$_2$Ge$_2$
Source: arXiv:1405.4007 source file (2016-02-04)
Supplement: Supplementary file 1 [file supplementalinfoarxivPRINT.pdf]

# Supplemental material for "Anomalous frequency and temperature dependent scattering and Hund's coupling in the almost quantum critical heavy fermion system $CeFe_2Ge_2$"

(Dated:)

## CONDUCTIVITY MEASUREMENTS AND FITTING ANALYSIS

Conductivity measurements were taken at temperatures between 1.55 K and room temperature in a continuous-flow liquid He-4 cryostat. Because of the large number of temperatures at which data was taken, displaying the complex conductivity as a function of frequency for all temperatures at once masks the details of the individual curves and was not shown in the main text. However, the systematic development of a narrow Drude peak in the real part of the conductivity as temperature is lowered is seen very nicely in this fashion. The real and imaginary parts of the complex conductivity are shown for the full temperature spectrum in Fig. 1. The data is cut to a frequency range of 200 GHz-1.5 THz. The dc conductivity points, calculated from the dc resistivity data taken using a 4-probe technique, are also shown as solid markers. Drude-Lorentz model fits, shown as dashed lines, were performed assuming there are no sharp features below 200 GHz and the dc value.

The Drude-Lorentz model fits were performed using the software RefFit [1]. This program is capable of fitting multiple complex valued datasets of different experimental types simultaneously with multiple models, which may depend on the same parameters. We fit the real and imaginary parts of our measured conductivity with a number of Drude-Lorentz style oscillators and produce a model of the dielectric function of our sample at each temperature taken. The parameters that can be adjusted in any generic model are the transverse frequency $\omega_0$, plasma frequency $\omega_p$ and linewidth $\gamma$ of each oscillator chosen to fit the data. There is also a high-frequency dielectric constant $\epsilon_\infty$, which represents the contributions of all oscillators at very high frequencies compared to the frequency range under consideration. We find that the THz spectral range can be fit very well with just two Drude ($\omega_0 = 0$) oscillators. We saw that the addition of more oscillators did not improve the fit significantly enough to justify their inclusion. All other parameters were adjustable. During the fit, the dc data point was given 10 times the weight of the THz data in order to ensure that the fit passes through the dc value.

## DETERMINATION OF THE FULL PLASMA FREQUENCY $\omega_p$

In our analysis, $\omega_p$ used in the extended Drude equations

$$\frac{m^*(\omega)}{m_b} = -\frac{\omega_p^2}{4\pi\omega} Im\left[\frac{1}{\sigma(\omega)}\right] \tag{1}$$

$$\frac{1}{\tau(\omega)} = \frac{\omega_p^2}{4\pi} Re\left[\frac{1}{\sigma(\omega)}\right] \tag{2}$$

must come from the spectral weight of the full intraband Drude contribution[2, 3]. To clarify this we start with the well know sum rule for optical conductivity

$$8\int_0^\infty \sigma_1(\omega) d\omega = \frac{4\pi N e^2}{m_e} \tag{3}$$

where $N$ is the total number of charges and $m_e$ is their mass. However, the integration extending to infinity presents a considerable experimental complication and the sum rule is usually restricted to a partial sum rule

$$8\int_0^W \sigma_1(\omega) d\omega = \frac{4\pi N e^2}{m_b} \tag{4}$$

where $W$ is the unrenormalized electronic bandwidth, $N$ is the number of mobile charge carriers and $m_b$ is the band mass. From this, we can define the plasma frequency $\omega_p^2 = \frac{4\pi N e^2}{m_b}$. If $W$ is sufficiently high enough we recover the full sum rule. For strongly interacting systems we can further limit the sum rule and perform the integration over an energy $E$ only several times the Drude width to determine the renormalized mass $m^*$ due to interactions

$$8\int_0^E \sigma_1(\omega) d\omega = \frac{4\pi N e^2}{m^*}. \tag{5}$$

In this case we can define a renormalized plasma frequency $\omega_p^{*2} = \frac{4\pi N e^2}{m^*}$, which only describes the spectral weight of a very narrow interaction derived band, not the full contribution described in Eq. 4. The ratio of these two plasma frequencies is often cited in the context of heavy fermion systems $\frac{\omega_p^2}{\omega_p^{*2}} = \frac{m^*}{m_b}$ to describe the large renormalization of the charge carrier mass due to hybridization of the band of conduction electrons with the localized band of magnetic moments.

The question remains: which plasma frequency should be used in the extended Drude model Eqs. 1, 2 ? Recall that the origin of the extended Drude model is to account for the various inelastic channels that contribute to

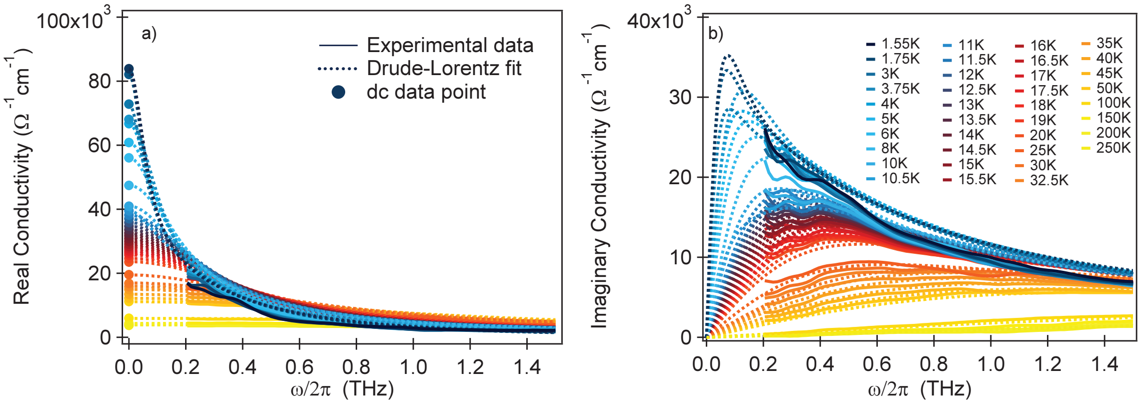


FIG. 1. (a) Real and (b) Imaginary parts of the complex conductivity for all temperatures.

the scattering rate with different frequency dependencies. While the Drude-Lorentz model treats the scattering rate of the intraband contribution as being characterized by a single frequency independent relaxation time, the extended Drude model captures these frequency dependencies by explicitly making the scattering rate and mass frequency dependent. Therefore, $\omega_p$ must come from the spectral weight of the full intraband contribution. In the context of sum rules,

$$8\int_0^\infty \sigma_1^{intra}(\omega)d\omega = \omega_p^2 \quad (6)$$

where $\sigma_1^{intra}$ represents the conductivity from all intraband contributions. Again, the intergration to infinity is usually replaced by a high energy cut-off that is large enough to capture all intraband transitions while minimizing the contaminating contribution of interband transitions. In our case, the plasma frequency that enters into the extended Drude model equations reflects both the spectral weight of the narrow Drude peak associated with the heavy charge carriers and the spectral weight of other higher frequency scattering processes.

To experimentally determine $\omega_p$ of CFG we performed Fourier transform infrared (FTIR) spectroscopy in transmission and reflection geometries from 100-8000 cm$^{-1}$ and with the THz data, we used the same modeling software, RefFit, to parameterize the spectra[1]. In the reflection geometry, the sample and substrate were mounted on top of gold mirrors and referenced to identical mirrors. A special function in RefFit that models a multilayer sample was chosen to fit the CFG thin film on an MgO substrate(special code -33). This function takes as input the models that parameterize the dielectric function of each layer and outputs the dielectric function of the composite system. By doing this, we are able to isolate the optical response of the CFG film.

An example of the fitting technique is seen in Fig. 2. The first step of the fitting analysis is to model the dielectric function of the MgO substrate and the gold mirror. Once this is known, these models are fixed and are not be adjusted during further fitting steps. Next, we create a "skeleton model" which will characterize the CFG layer. For this we separate the oscillators into low-frequency Drude and Drude-Lorentz terms, which characterize the intraband transitions, and higher frequency Drude-Lorentz oscillators, which characterize interband transitions. The plasma frequencies associated with the intraband terms are then added in quadrature to determine $\omega_p$ that we will use in the extended Drude model calculations. Finally, we create another model, which is specially designed for multilayer systems (special code -33). The normal parameters of any generic model are reassigned in this model: each row in the model represents a layer of the system. There are actually two of these models- one for transmission and another for reflection fitting. We can now fit these models to the CFG + MgO multilayer FTIR transmission data, the CFG+MgO+gold FTIR reflection data and the THz conductivity data. The only parameters free to fit are in the CFG layer model. The self-consistent results of this modeling technique are shown in Fig. 3. The FTIR reflection and transmission data are shown with the multilayer parameterizations of the data. The model that parameterizes the CFG layer is also shown with TDTS data to show the consistency between parameterization of the FTIR and TDTS data.

The main source of error in determining $\omega_p$ within this fitting technique arises from distinguishing at what frequency the influence of interband transitions begins to contaminate the low-frequency physics we are most interested in. To quantify this error we took our best model and split a "mid-frequency" oscillator (1500 cm$^{-1}$), which had a very broad scattering rate, into two oscillators: one at a lower frequency with a sharper scattering rate and the other at a higher frequency with a broad scattering rate. By doing this, the distribution of the spectral weight of the original oscillator is now more eas-

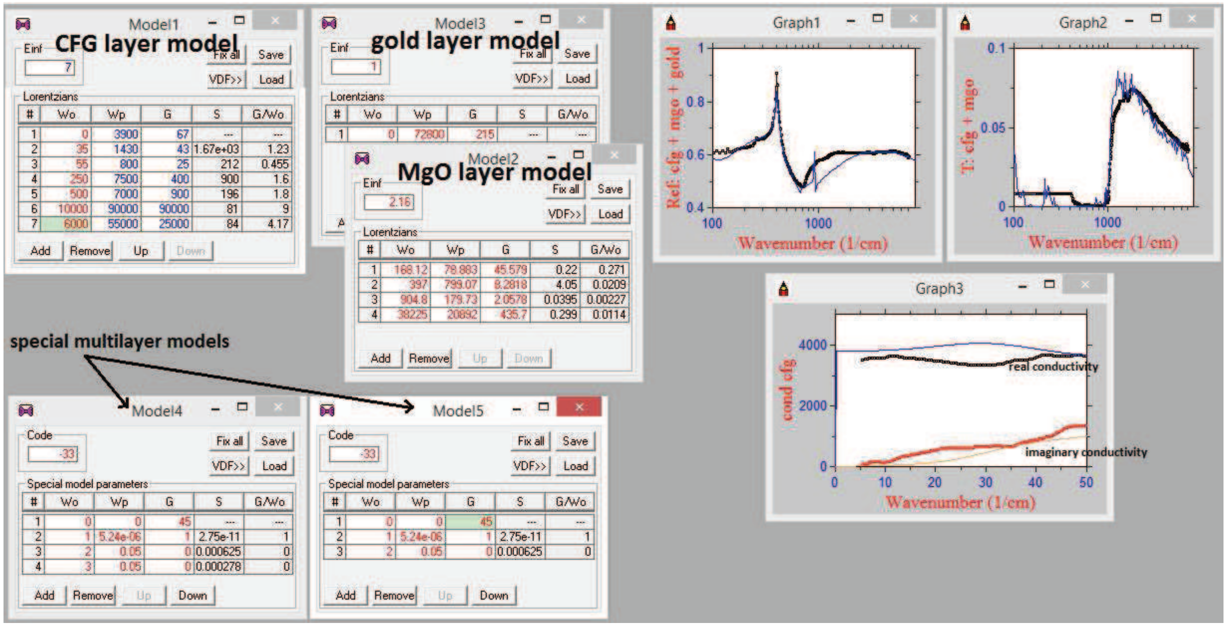


FIG. 2. A screenshot of the fitting program, RefFit, used to determine $\omega_p$ of CFG. A special multilayer model is necessary to fit the FTIR reflection and transmission data.

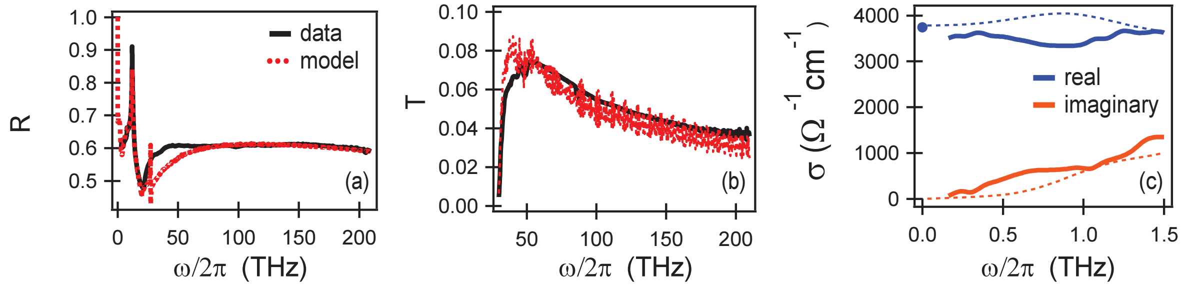


FIG. 3. (a)Reflection as a function of frequency for the CFG thin film grown on MgO, mounted on top of a gold substrate. The solid line is FTIR data; the dashed line is the result of a multilayer parameterization of this data. (b) Transmission as a function of frequency for the CFG thin film grown on MgO. The solid line is FTIR data; the dashed line is the result of a multilayer parameterization of this data. (c)Real and imaginary parts of the complex conductivity of CFG. Solid lines are data taken using TDTS. Dashed lines represent models of the CFG layer within the multilayer parameterizations shown in (a) and (b).

ily identified with either intra or interband transitions while the quality of the fit is maintained.

Deciding how to separate low(intraband) from high(interband) frequency processes is motivated from previous work done on similar compounds [4][5]. Two methods are commonly used: 1) the frequency at which there is a minimum in the real part of the conductivity and 2) the frequency at which the imaginary part of the conductivity crosses from positive to negative. At these frequencies the influence of interband processes dominates the Drude response. Instrument and sample limitations do not allow us to measure the conductivity directly beyond the THz regime, but the model that we generate using Reffit shows these features and confirms our belief that the cut-off energy scale in CFG is $\sim$3000 cm$^{-1}$. This is similar to other Fe based materials with the same crystal structure [4][5]. Table I shows the original model with all oscillators and the final model after splitting the oscillator at 1500 cm$^{-1}$. Table II gives more detail about this splitting process. It is seen in this table that an acceptable range of plasma frequencies to characterize the lower intraband oscillator is $\sim$7000-10000 cm$^{-1}$ since their scattering rates are sufficiently narrow that most of their spectral weight still lies below the high energy cut-off of $\sim$3000 cm$^{-1}$. Using this range and adding the spectral weight of the oscillators centered below 3000 cm$^{-1}$ in quadrature we determine $\omega_p$ = 12150 $\pm$ 1000 cm$^{-1}$.

| original model | | | |
|---|---|---|---|
| type | $\omega_o$ | $\omega_p$ | $\Gamma$ |
| intraband | 0 | 3900 | 67 |
| intraband | 40 | 1200 | 65 |
| intraband | 60 | 1755 | 50 |
| intraband | 250 | 7500 | 400 |
| ? | 1500 | 25500 | 8000 |
| interband | 6000 | 55000 | 25000 |

| final model | | | |
|---|---|---|---|
| type | $\omega_o$ | $\omega_p$ | $\Gamma$ |
| intraband | 0 | 3900 | 67 |
| intraband | 40 | 1200 | 65 |
| intraband | 60 | 1755 | 50 |
| intraband | 250 | 7500 | 400 |
| intraband | 500 | 7000-10000 | 800-3500 |
| interband | 2500+ | 29000+ | 14000+ |
| interband | 6000 | 55000 | 25000 |

TABLE I. The original model that fit the data very well, but had an oscillator centered at 1500 cm$^{-1}$ that was not well defined as originating from intraband or interband transitions. To provide a better assignment of spectral weight we split this ambiguous oscillator into two (see Table II for details). All units are cm$^{-1}$.

| splitting of 1500 cm$^{-1}$ osc. | | |
|---|---|---|
| $\omega_o$ | $\omega_p$ | $\Gamma$ |
| 1500 | 25500 | 8000 |
| 1500<br>1500 | 18000<br>18000 | 8000<br>8000 |
| 1000<br>2000 | 14000<br>24000 | 6500<br>12000 |
| 500<br>2500 | 10000<br>29000 | 3500<br>14000 |
| 500<br>4000 | 8000<br>3400 | 1300<br>18000 |
| 500<br>6000 | 7000<br>54000 | 1000<br>34000 |
| 500<br>8000 | 7000<br>70000 | 1000<br>55000 |
| 500<br>10000 | 7000<br>90000 | 900<br>90000 |

TABLE II. Details of how the broad oscillator, originally centered at 1500 cm$^{-1}$, was split and its spectral weight was redistributed. All units are cm$^{-1}$.

## EXTENDED DRUDE MODEL ANALYSIS

Fits to the renormalized scattering rate and mass were also performed using RefFit software[1]. A built-in function (special code -6) specifically designed for the extended Drude model takes as input a dielectric function $\epsilon(\omega)$ given by the dielectric model calculated previously in our conductivity fitting and converts it to the frequency-dependent scattering rate and effective mass according to the formulas

$$\frac{m^*(\omega)}{m_b} = -\frac{\omega_p^2}{\omega^2} Re\left[\frac{1}{\epsilon(\omega)-\epsilon_\infty}\right] \tag{7}$$

$$\frac{1}{\tau(\omega)} = -\frac{\omega_p}{\omega} Im\left[\frac{1}{\epsilon(\omega)-\epsilon_\infty}\right] \tag{8}$$

where $\omega_p$ is the full plasma frequency obtained using Fourier transform infrared spectroscopy. This parameter describes the high frequency spectral weight that represents the spectral weight from all free carriers and is not to be confused with the narrowest low frequency Drude plasma frequency, which is commonly associated with the heavy charge carriers. Further discussion of this parameter is described elsewhere in the Supplemental Material. $\epsilon_\infty$, as previously discussed, represents the contributions of all oscillators at very high frequencies. It should be noted that $\omega_p$ and $\epsilon_\infty$ used in this model are not the same as the parameters of the RefFit model used to calculate $\epsilon(\omega)$. An example of this fitting process is seen in Fig. 4.

The extended Drude model fits are essential to determining the zero frequency limit of the renormalized mass. From the THz data alone one would not conclude that a large mass renormalization takes place. However, with the combination of the THz data AND the dc resistivity data along with an extended Drude model fit, it is possible to infer how the mass renormalization changes as one connects the THz data to the dc data. The extended Drude model applied to the two Drude oscillator fits allows us to make this connection within a model that only depends on the Kramers-Kronig transform. Of course the exact shape of the frequency dependence in the range where there is no data should not be believed, but the general dependence of going from the high mass value at low $\omega$ to the low mass at high $\omega$ will be correct.

## SCATTERING RATE POWER LAW FITS

A full view of the scattering rate as a function of frequency for all temperatures is shown in Fig. 5. It is clear that the scattering rate is systematically suppressed as the temperature is lowered. It is difficult, when looking at all the spectra at once, to notice frequency dependence to any individual curve. However, a frequency dependence does begin to form for temperatures below ∼15 K. To quantify this dependence we chose to fit the scattering rates to a simple power law $\frac{1}{\tau(\omega,T)} = \frac{1}{\tau(0,T)} + A\omega^n$. The frequency range we fit over had a noticeable influence on the exponent calculated. To account for this, we fit over a few different frequency ranges (i.e 0.2-1.25 THz, 0.2-1.5 THz, 0.2-1.75 THz) and average the calculated exponents.

In certain cases, the values of the $A$ coefficient in the simple power law fits to the scattering rate can be used

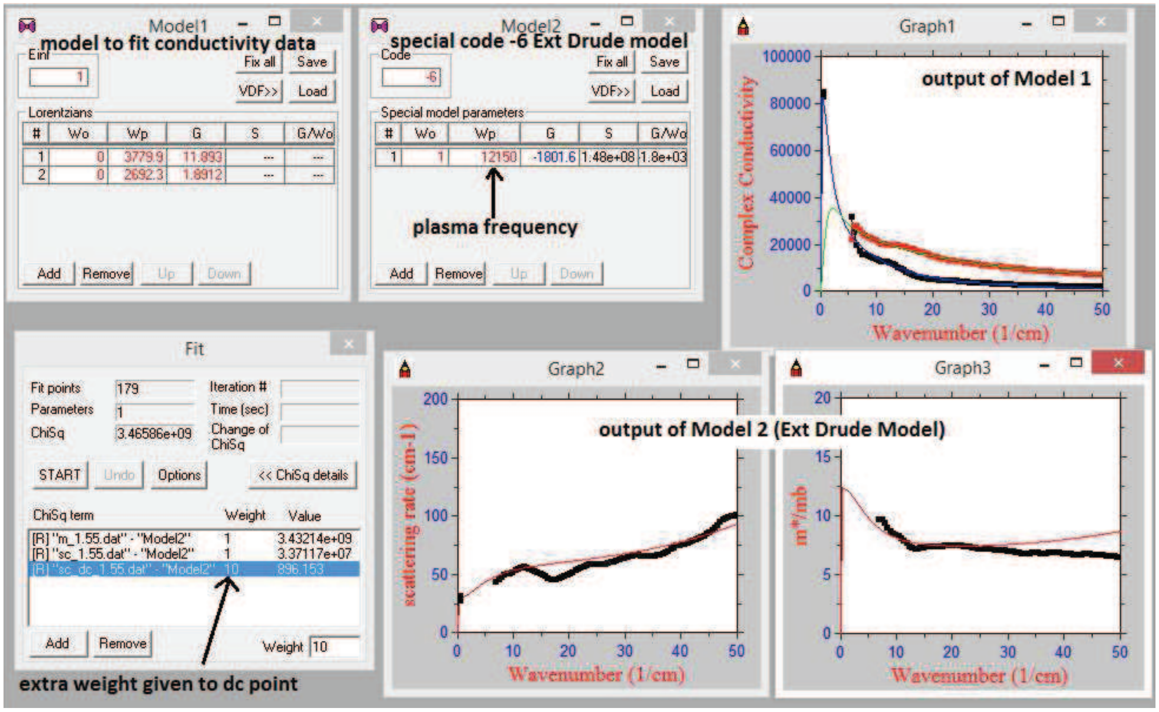


FIG. 4. A screenshot of the fitting program, RefFit, used to perform the extended Drude model fits on the previously calculated optical conductivity models.

in a further analysis of the heavy fermion state. For example, when the frequency dependence of the scattering rate goes like $\omega^2$, the $A$ coefficient can be used in a Kadowaki-Woods-like analysis[6]. However, because we find that our exponent in the power law is changing with temperature, we are not able to carry out such an analysis. Because the exponent is changing at every temperature, the units of the $A$ coefficient are also changing at every temperature. This makes a strict comparison of the $A$ coefficients as a function of temperature meaningless. For completeness, though, the $A$ coefficients extracted from the best power law fit to the scattering rate can be found in Table III.

To determine the error bars on the exponents extracted from the power law fits, we use $\chi^2$ values to estimate the range of exponents that produce fits of comparable quality. We fit the scattering rate at each temperature below 12 K over three frequency ranges (0.2-1.25 THz, 0.2-1.5 THz, 0.2-1.75 THz) to a simple power law, holding the exponent to fixed value (0.50, 0.55,..., 2.50) and record the corresponding $\chi^2$ values. Then, we find the minimum in the $\chi^2$ values $\pm 10\%$ to get a range of exponents that produce fits of similar quality. The error bars seen in Fig. 3c of the manuscript correspond to the range of exponents for each individual temperature. Fig. 6 shows $\chi^2$ vs. $n$, the exponent in the power law fits, for temperatures below 12 K for fits done over the frequency range 0.2-1.5 GHz. Similar results were seen in the fits performed over the frequency ranges 0.2-1.25 GHz and 0.2-1.75 GHz. Table III shows the value of the exponents for temperatures below 12K. The reasonable sensitive dependence of $\chi^2$ on the fitting exponent gives us confidence in the veracity of our approach.

[1] A. B. Kuzmenko, Rev. Sci. Instrum. **76**, 083108 (2005).
[2] L. Degiorgi, Rev. Mod. Phys. **71**, 687 (1999).
[3] N. P. Armitage, arXiv:0908.1126.
[4] A. A. Schafgans, et. al, Phys. Rev. Lett. **108**, 147002
[5] A. A. Schafgans, et. al, `http://link.aps.org/supplemental/10.1103/PhysRevLett.108.147002`
[6] K. Kadowaki and S. B. Woods, Solid State Communications **58**, 507 (1986)

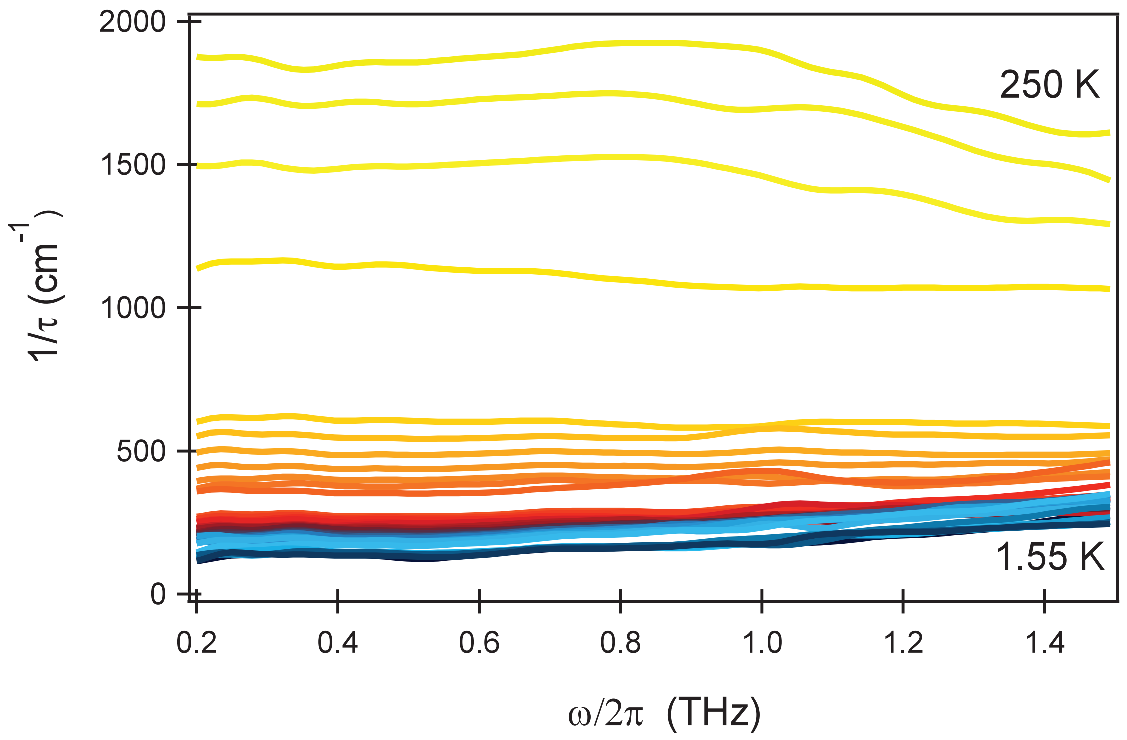


FIG. 5. Scattering rate as a function of frequency for all temperatures 1.55-250 K.

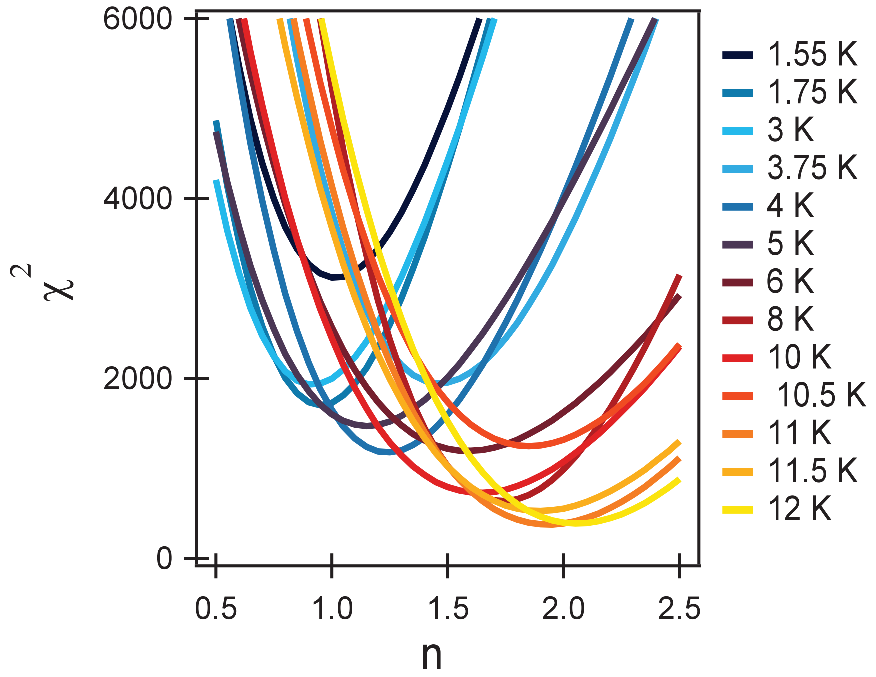


FIG. 6. $\chi^2$ vs. $n$, the exponent in the simple power law fit to the scattering rate performed over the frequency range 0.2-1.5 GHz for temperatures below 12 K. Similar results were obtained for fits performed over the frequency ranges 0.2-1.25 GHz and 0.2-1.75 GHz.

| Temp (K) | $n$ (fit range: 0.2-1.25 THz) | $n$ (fit range: 0.2-1.5 THz) | $n$ (fit range: 0.2-1.75 THz) | Average $n$ | $A$ coefficient |
|---|---|---|---|---|---|
| 1.55 | 0.660 | 0.991 | 1.21 | 0.955 | 40.8 |
| 1.75 | 0.835 | 0.950 | 0.965 | 0.916 | 40.4 |
| 3 | 0.695 | 0.905 | 0.946 | 0.849 | 37.5 |
| 3.75 | 1.11 | 1.45 | 1.34 | 1.30 | 39.3 |
| 4 | 1.10 | 1.23 | 1.37 | 1.23 | 35.5 |
| 5 | 0.883 | 1.13 | 1.24 | 1.09 | 30.5 |
| 6 | 1.26 | 1.59 | 1.30 | 1.38 | 26.4 |
| 8 | 1.65 | 1.73 | 1.78 | 1.72 | 36.5 |
| 10 | 1.40 | 1.64 | 1.63 | 1.56 | 26.4 |
| 10.5 | 1.74 | 1.87 | 1.71 | 1.77 | 28.3 |
| 11 | 1.89 | 1.93 | 1.83 | 1.88 | 25.0 |
| 11.5 | 1.87 | 1.89 | 1.85 | 1.87 | 25.0 |
| 12 | 2.19 | 2.06 | 1.97 | 2.07 | 26.1 |

TABLE III. The exponent, $n$, and the $A$ coefficient from fitting the scattering rate as a function of frequency using a simple power law over three frequency ranges.
